# Supplementary material for: Estimating Group Average Treatment Effects in High-Risk Populations with Unobserved Target Membership
Source: arXiv:2610.30709 source file (2026-10-22)
Supplement: Supplementary file 1 [file Supplementary.tex]

\documentclass[11pt,letterpaper]{article}
\input{latex/arXiv/Supplementary.tex}
